# Supplementary material for: Statistical limits of dictionary learning: random matrix theory and the spectral replica method
Source: arXiv:2109.06610 source file (2022-02-26)
Supplement: Supplementary file 1 [file AppendixIntegrals.tex]

\section{Integrals and moments}

\subsection{The Tricomi formula}

We calculate distribution $d\rho_s(y)$ from the Tricomi formula
$$
\rho_\Sigma(y) = \frac{1}{\pi\sqrt{(y-a)(y-b)}}\Big(C - \int_a^b \frac{dx}{\pi} \frac{\sqrt{(x-a)(x-b)}}{y -x} G^\prime(x)\Big)
$$
for $G^\prime(x) = \frac{G_{-1}}{x} + G_0 + G_1 x + G_2 x^2 + G_3 x^3$. In order for this formula to be valid it is assumed that 
the distribution has support $[a, b]$.

Recall the notation $m= \frac{a+b}{2}$, $s= \frac{b-a}{2}$. We define for $p=-1, 0, 2, 3, \cdots$
$$
I_p(y) = \int_a^b \frac{dx}{\pi}  \frac{\sqrt{(x-a)(b-x)}}{y-x} x^p .
$$
Then 
$$
\rho_\Sigma(y) = \frac{1}{\pi\sqrt{(y-a)(y-b)}}\Big(C - G_{-1} I_{-1}(y)  - G_0 I_0(y) - G_1 I_1(y) - G_2 I_2(y) - G_3 I_3(y) + \cdots\Big)
$$
According to \cite{Giang} we have 
$$
I_0(y) = ( y -m) + (\mathds{1}(y < a) - \mathds{1}(y > b)) \sqrt{((y - a)( y-b)}
$$
Furthermore we note
\begin{align*}
I_{-1}(y) & = \frac{1}{y} \int_a^b \frac{dx}{\pi}  \sqrt{(x-a)(b-x)} \biggl(\frac{1}{y-x} + \frac{1}{x}\biggr)
\nonumber \\ &
=
\frac{I_0(y) - I_0(0)}{y}
\nonumber \\ &
=
1 + \frac{(\mathds{1}(y< a) - \mathds{1}(y>b)) \sqrt{(y-a)(y-b)}}{y} - \frac{(\mathds{1}(0< a) - \mathds{1}(0>b)) \sqrt{ab}}{y}
\end{align*}

Now for $p\ge1$ we have 
\begin{align*}
I_p(y) & = - \int_a^b \frac{dx}{\pi}  \frac{\sqrt{(x-a)(b-x)}}{y-x} (y^p - x^p) + y^p \int_a^b \frac{dx}{\pi}  \frac{\sqrt{(x-a)(b-x)}}{y-x} 
\nonumber \\ &
=
- \int_a^b \frac{dx}{\pi}  \sqrt{(x-a)(b-x)} \sum_{k=0}^{p-1} x^{k} y^{p-1 -k} + y^p I_0(y)
\nonumber \\ &
=
-  \sum_{k=0}^{p-1} y^{p-1 -k} \int_a^b \frac{dx}{\pi}  \sqrt{(x-a)(b-x)} x^{k} + y^p I_0(y)
\end{align*}
Now we use the changes of variables $y = m + z$ and $z = s \cos\theta$ and find
\begin{align*}
\int_a^b \frac{dx}{\pi}  \sqrt{(x-a)(b-x)} x^{k}  & = \int_{-s}^s \frac{dz}{\pi}  \sqrt{s^2  - z^2} (m + z)^{k} 
\nonumber \\ &
=
s^2 \int_{\pi}^{2\pi} \frac{d\theta}{\pi} (\sin\theta)^2 (m+ s \cos\theta)^k
\nonumber \\ &
=  s^2 \sum_{\ell =0}^{k} \binom{k}{\ell} s^\ell m^{k-\ell} \int_{\pi}^{2\pi} \frac{d\theta}{\pi} (\sin\theta)^2 (\cos\theta)^\ell
\nonumber \\ &
=  s^2 \sum_{\ell =0}^{k} \binom{k}{\ell} s^\ell m^{k-\ell} \bigg\{\int_{0}^{2\pi} \frac{d\theta}{2\pi} (\cos\theta)^\ell - \int_{\pi}^{2\pi} \frac{d\theta}{\pi} (\cos\theta)^{\ell +2}\biggr\}
\nonumber \\ &
=  s^2 \sum_{\ell= 0, \cdots, k: {\rm \, even}} \binom{k-1}{\ell} \left(\frac{s}{2}\right)^\ell m^{k-\ell} \bigg\{\binom{\ell}{\frac{\ell}{2}} 
- \frac{1}{4}\binom{\ell + 2}{\frac{\ell}{2} + 1} \biggr\}
\end{align*}
Thus finally 
\begin{align*}
I_p(y) = & 
y^p\Bigl\{( y -m) + (\mathds{1}(y < a) - \mathds{1}(y > b)) \sqrt{((y - a)( y-b)}   \Bigr\}
\nonumber \\ &
-  s^2 \sum_{k=0}^{p-1} y^{p-1 -k} 
\sum_{\ell= 0, \cdots, k: {\rm \, even}} \binom{k}{\ell} \left(\frac{s}{2}\right)^\ell m^{k-\ell} \bigg\{\binom{\ell}{\frac{\ell}{2}} 
- \frac{1}{4}\binom{\ell + 2}{\frac{\ell}{2} + 1} \biggr\}
\end{align*}
We find 
$$
I_1(y) = y \Bigl\{( y -m) + (\mathds{1}(y < a) - \mathds{1}(y > b)) \sqrt{((y - a)( y-b)}   \Bigr\} - \frac{s^2}{2}
$$
$$
I_2(y) = y^2 \Bigl\{( y -m) + (\mathds{1}(y < a) - \mathds{1}(y > b)) \sqrt{((y - a)( y-b)}   \Bigr\} - y \frac{s^2}{2} - \frac{ms^2}{2}
$$
$$
I_3(y) = y^2 \Bigl\{( y -m) + (\mathds{1}(y < a) - \mathds{1}(y > b)) \sqrt{((y - a)( y-b)}   \Bigr\}  -  y^2 \frac{s^2}{2} - y \frac{m s^2}{2} 
- ( \frac{m^2s^2}{2} + \frac{s^4}{8})
$$
Our final result is then 
\begin{align*}
\rho_\Sigma(y) = & \frac{1}{\pi\sqrt{(y-a)(y-b)}}
\Biggl\{ C - G_{-1}\Big( 1 + \frac{(\mathds{1}(y< a) - \mathds{1}(y>b)) \sqrt{(y-a)(y-b)}}{y} - \frac{(\mathds{1}(0< a) - \mathds{1}(0>b)) \sqrt{ab}}{y}\Big)
\nonumber \\ &
- (G_0 + G_1 y + G_2 y^2 + G_3 y^3)\biggl\{(y-m) +  (\mathds{1}(y < a) - \mathds{1}(y > b)) \sqrt{((y - a)( y-b)} \biggr\}
\nonumber \\ &
+ (G_1 \frac{s^2}{2} + G_2 \frac{ms^2}{2} + G_3 (\frac{m^2s^2}{2} + \frac{s^4}{8})) + y (G_2 \frac{s^2}{2} + G_3 \frac{ms^2}{2}) + y^2 G_3 \frac{s^2}{2}
\Bigg\}
\end{align*}

This expression can be simplified using $a\leq y \leq b$. This yields after some reorganisation of the terms
\begin{align*}
\rho_\Sigma(y) = & 
\frac{1}{\pi\sqrt{(y-a)(y-b)}}
\Biggl\{ G_{-1} \frac{(\mathds{1}(0< a) - \mathds{1}(0>b)) \sqrt{ab}}{y} 
\nonumber \\ & 
+ \Bigl( C - G_{-1} + G_0 m + G_1 \frac{s^2}{2} + G_2 \frac{ms^2}{2} + G_3 (\frac{m^2s^2}{2} + \frac{s^4}{8})\Bigr)
+ y\Bigl( - G_0 + G_1 m + G_2 \frac{s^2}{2} + G_3 \frac{ms^2}{2}\Bigr)
\nonumber  \\ &
+ y^2 \Bigl( - G_1 + G_2 m + G_3 \frac{s^2}{2} \Bigr)
+ y^3 (- G_2 + G_3m) - y^4 G_3
\Biggr\}
\end{align*}

\subsection{Some useful moments}

Define the normalized measure
$$
d(y) = \frac{1}{\pi \sqrt{((y-a) (b-y)}}, \quad a\leq y \leq b .
$$
We compute the moments $d_p = \int_a^b dy\, y^p d(y)$. 

Consider the change of variable $y\to z$ such that $y = m + z$. We have 
\begin{align}
d_p & = \int_a^b dy \frac{y^p}{\pi \sqrt{((y-a) (b-y)}} = \int_{-s}^s dz \frac{(m+z)^p}{\pi \sqrt{s^2 - z^2}}
\\ \nonumber &
=
\int_0^\pi \frac{d\theta}{\pi} (m + s \cos\theta)^p = \sum_{\ell=0}^p \binom{p}{\ell} m^\ell s^{p-\ell} \int_0^{2\pi} \frac{d\theta}{2\pi} (\cos\theta)^{p-\ell}
\\ \nonumber &
= \sum_{\ell=0\cdots p {\rm \, \,} p-\ell {\rm \,\, even}} \binom{p}{\ell} \binom{p-\ell}{\frac{p-\ell}{2}} m^\ell s^{p-\ell} \frac{1}{2^{p-\ell}}
\end{align}
where the last equality comes from 
\begin{align}
\int_0^{2\pi} \frac{d\theta}{2\pi} (\cos\theta)^{p-\ell} & = \frac{1}{2^{p-\ell}} \sum_{k=0}^{p-\ell} \binom{p}{k}\int_0^{2\pi} \frac{d\theta}{2\pi}  e^{i\theta k} e^{- i\theta(p-\ell -k)}
\nonumber \\ &
= \frac{1}{2^{p-\ell}} \sum_{k=0}^{p - \ell} \binom{p}{k}\int_0^{2\pi} \frac{d\theta}{2\pi}   e^{i\theta (2k- (p- \ell)))}
\nonumber \\ &
= 
\begin{cases}
\frac{1}{2^{p-\ell}} \binom{p-\ell}{\frac{p-\ell}{2}}, \quad p-\ell {\rm \, even}\\
0, 
\quad p-\ell {\rm \, odd}
\end{cases}
\end{align}
The special cases that interest us are $d_0 =1$ (normalization of the measure), $d_1 = m$, $d_2 = \frac{s^2}{2} + m^2$, $d_3 = \frac{3}{2}ms^2 + m^3$, $d_4 = \frac{3}{8}s^4 + 3m^2s^2 + m^4$, $d_5 =  \frac{15}{8} m s^4 + 5 m^3 s^2 + m^5$, $d_6= \frac{5}{16} s^6 + \frac{45}{8} m^2 s^4 + \frac{15}{2} m^4 s^2 + m^6$, $d_7 =  \frac{35}{32} m s^6 + \frac{105}{8} m^3 s^4 + \frac{21}{2} m^5 s^2 + m^7$.

We also need the result  from \cite{Giang}
$$
d_{-1} = \int_a^b dy \frac{y^{-1}}{\pi \sqrt{((y-a) (b-y)}} = \frac{1}{\sqrt{ab}} ( \mathds{1}(a > 0) - \mathds{1}(b<0))
$$
We note the interesting fact that this vanishes for all intervals such that $a>0$ and $b<0$.
